# Supplementary material for: Precision measurement of charged pion and kaon differential cross sections in electron-positron annihilation at Q = 10.52 GeV
Source: arXiv:1301.6183 ancillary file (2013-08-09)
Supplement: Supplementary file 1 [file Supplemental_ChargedDiffCrossSections_PRL_v1.43_070213.pdf]

**Supplemental Document to Manuscript**  
**Precision measurement of charged pion and kaon differential cross sections in  $e^+e^-$**   
**annihilation at  $\sqrt{s} = 10.52$  GeV**

**CHARGE-INTEGRATED DIFFERENTIAL PION PRODUCTION CROSS SECTIONS**

Low  $z = 2E_h/\sqrt{s}$  bin limit (inclusive, constant bin width  $\Delta z = 0.01$ ), cross section value  $d\sigma_{\pi^\pm}/dz$  [fb], statistical uncertainty, positive systematic uncertainty, negative systematic uncertainty. The uncertainties do not include the uncertainty on the normalization constant (1.4%).

|      |               |           |             |             |
|------|---------------|-----------|-------------|-------------|
| 0.20 | 2.03779e + 07 | 7.0e + 03 | 3.846e + 05 | 3.844e + 05 |
| 0.21 | 1.83246e + 07 | 6.6e + 03 | 3.562e + 05 | 3.560e + 05 |
| 0.22 | 1.65093e + 07 | 6.3e + 03 | 3.318e + 05 | 3.317e + 05 |
| 0.23 | 1.48789e + 07 | 5.9e + 03 | 2.964e + 05 | 2.963e + 05 |
| 0.24 | 1.34435e + 07 | 5.6e + 03 | 2.769e + 05 | 2.768e + 05 |
| 0.25 | 1.21936e + 07 | 5.4e + 03 | 2.570e + 05 | 2.569e + 05 |
| 0.26 | 1.10808e + 07 | 5.1e + 03 | 2.428e + 05 | 2.427e + 05 |
| 0.27 | 1.00835e + 07 | 4.9e + 03 | 2.229e + 05 | 2.228e + 05 |
| 0.28 | 9.1788e + 06  | 4.6e + 03 | 2.071e + 05 | 2.070e + 05 |
| 0.29 | 8.3661e + 06  | 4.4e + 03 | 1.906e + 05 | 1.906e + 05 |
| 0.30 | 7.6396e + 06  | 4.2e + 03 | 1.876e + 05 | 1.876e + 05 |
| 0.31 | 6.9893e + 06  | 4.0e + 03 | 1.774e + 05 | 1.774e + 05 |
| 0.32 | 6.4020e + 06  | 3.8e + 03 | 1.652e + 05 | 1.651e + 05 |
| 0.33 | 5.8605e + 06  | 3.7e + 03 | 1.553e + 05 | 1.553e + 05 |
| 0.34 | 5.3715e + 06  | 3.5e + 03 | 1.493e + 05 | 1.492e + 05 |
| 0.35 | 4.9245e + 06  | 3.4e + 03 | 1.340e + 05 | 1.339e + 05 |
| 0.36 | 4.5227e + 06  | 3.2e + 03 | 1.242e + 05 | 1.241e + 05 |
| 0.37 | 4.1513e + 06  | 3.1e + 03 | 1.177e + 05 | 1.177e + 05 |
| 0.38 | 3.8135e + 06  | 2.9e + 03 | 1.087e + 05 | 1.086e + 05 |
| 0.39 | 3.5043e + 06  | 2.8e + 03 | 1.042e + 05 | 1.041e + 05 |
| 0.40 | 3.2246e + 06  | 2.7e + 03 | 9.56e + 04  | 9.55e + 04  |
| 0.41 | 2.9715e + 06  | 2.6e + 03 | 8.95e + 04  | 8.95e + 04  |
| 0.42 | 2.7383e + 06  | 2.5e + 03 | 8.40e + 04  | 8.39e + 04  |
| 0.43 | 2.5296e + 06  | 2.4e + 03 | 7.94e + 04  | 7.94e + 04  |
| 0.44 | 2.3378e + 06  | 2.3e + 03 | 7.65e + 04  | 7.65e + 04  |
| 0.45 | 2.1578e + 06  | 2.2e + 03 | 6.83e + 04  | 6.83e + 04  |
| 0.46 | 1.9970e + 06  | 2.1e + 03 | 6.55e + 04  | 6.55e + 04  |
| 0.47 | 1.8432e + 06  | 2.0e + 03 | 5.78e + 04  | 5.78e + 04  |
| 0.48 | 1.7076e + 06  | 2.0e + 03 | 5.78e + 04  | 5.78e + 04  |
| 0.49 | 1.5817e + 06  | 1.9e + 03 | 5.31e + 04  | 5.31e + 04  |
| 0.50 | 1.4648e + 06  | 1.8e + 03 | 4.92e + 04  | 4.92e + 04  |
| 0.51 | 1.3568e + 06  | 1.7e + 03 | 4.78e + 04  | 4.78e + 04  |
| 0.52 | 1.2565e + 06  | 1.7e + 03 | 4.41e + 04  | 4.41e + 04  |
| 0.53 | 1.1630e + 06  | 1.6e + 03 | 4.08e + 04  | 4.08e + 04  |
| 0.54 | 1.0786e + 06  | 1.6e + 03 | 3.94e + 04  | 3.94e + 04  |
| 0.55 | 1.001e + 06   | 1.5e + 03 | 3.88e + 04  | 3.88e + 04  |
| 0.56 | 9.273e + 05   | 1.4e + 03 | 3.54e + 04  | 3.54e + 04  |
| 0.57 | 8.598e + 05   | 1.4e + 03 | 3.28e + 04  | 3.28e + 04  |
| 0.58 | 7.973e + 05   | 1.3e + 03 | 3.26e + 04  | 3.26e + 04  |
| 0.59 | 7.405e + 05   | 1.3e + 03 | 2.95e + 04  | 2.95e + 04  |

|      |              |           |             |             |
|------|--------------|-----------|-------------|-------------|
| 0.60 | 6.872e + 05  | 1.2e + 03 | 2.78e + 04  | 2.78e + 04  |
| 0.61 | 6.376e + 05  | 1.2e + 03 | 2.69e + 04  | 2.68e + 04  |
| 0.62 | 5.936e + 05  | 1.2e + 03 | 2.40e + 04  | 2.40e + 04  |
| 0.63 | 5.512e + 05  | 1.1e + 03 | 2.37e + 04  | 2.37e + 04  |
| 0.64 | 5.117e + 05  | 1.1e + 03 | 2.17e + 04  | 2.16e + 04  |
| 0.65 | 4.737e + 05  | 1.0e + 03 | 1.96e + 04  | 1.96e + 04  |
| 0.66 | 4.415e + 05  | 1.0e + 03 | 2.03e + 04  | 2.02e + 04  |
| 0.67 | 4.1023e + 05 | 9.7e + 02 | 1.947e + 04 | 1.945e + 04 |
| 0.68 | 3.8041e + 05 | 9.4e + 02 | 2.055e + 04 | 2.053e + 04 |
| 0.69 | 3.5389e + 05 | 9.1e + 02 | 1.621e + 04 | 1.616e + 04 |
| 0.70 | 3.2841e + 05 | 8.8e + 02 | 1.693e + 04 | 1.688e + 04 |
| 0.71 | 3.0322e + 05 | 8.5e + 02 | 1.685e + 04 | 1.680e + 04 |
| 0.72 | 2.8126e + 05 | 8.2e + 02 | 1.504e + 04 | 1.498e + 04 |
| 0.73 | 2.5943e + 05 | 7.9e + 02 | 1.531e + 04 | 1.526e + 04 |
| 0.74 | 2.4048e + 05 | 7.6e + 02 | 1.441e + 04 | 1.436e + 04 |
| 0.75 | 2.2180e + 05 | 7.4e + 02 | 1.359e + 04 | 1.354e + 04 |
| 0.76 | 2.0364e + 05 | 7.1e + 02 | 1.285e + 04 | 1.279e + 04 |
| 0.77 | 1.8785e + 05 | 6.8e + 02 | 1.197e + 04 | 1.191e + 04 |
| 0.78 | 1.7218e + 05 | 6.6e + 02 | 1.101e + 04 | 1.095e + 04 |
| 0.79 | 1.5772e + 05 | 6.3e + 02 | 1.079e + 04 | 1.073e + 04 |
| 0.80 | 1.4466e + 05 | 6.1e + 02 | 1.089e + 04 | 1.084e + 04 |
| 0.81 | 1.3155e + 05 | 5.9e + 02 | 1.124e + 04 | 1.119e + 04 |
| 0.82 | 1.1962e + 05 | 5.7e + 02 | 8.86e + 03  | 8.81e + 03  |
| 0.83 | 1.0823e + 05 | 5.4e + 02 | 1.053e + 04 | 1.050e + 04 |
| 0.84 | 9.672e + 04  | 5.2e + 02 | 8.09e + 03  | 8.06e + 03  |
| 0.85 | 8.609e + 04  | 4.9e + 02 | 8.29e + 03  | 8.27e + 03  |
| 0.86 | 7.614e + 04  | 4.7e + 02 | 7.91e + 03  | 7.90e + 03  |
| 0.87 | 6.738e + 04  | 4.5e + 02 | 7.26e + 03  | 7.26e + 03  |
| 0.88 | 5.811e + 04  | 4.2e + 02 | 6.96e + 03  | 6.96e + 03  |
| 0.89 | 4.915e + 04  | 3.9e + 02 | 7.70e + 03  | 7.71e + 03  |
| 0.90 | 4.200e + 04  | 3.7e + 02 | 6.37e + 03  | 6.38e + 03  |
| 0.91 | 3.497e + 04  | 3.5e + 02 | 4.99e + 03  | 5.01e + 03  |
| 0.92 | 2.946e + 04  | 3.3e + 02 | 6.14e + 03  | 6.16e + 03  |
| 0.93 | 2.470e + 04  | 3.2e + 02 | 4.80e + 03  | 4.82e + 03  |
| 0.94 | 1.915e + 04  | 2.9e + 02 | 5.40e + 03  | 5.42e + 03  |
| 0.95 | 1.376e + 04  | 2.8e + 02 | 3.74e + 03  | 3.76e + 03  |
| 0.96 | 9.91e + 03   | 2.9e + 02 | 4.91e + 03  | 4.93e + 03  |
| 0.97 | 1.170e + 04  | 5.4e + 02 | 6.43e + 03  | 6.48e + 03  |

### CHARGE-INTEGRATED DIFFERENTIAL KAON PRODUCTION CROSS SECTIONS

Low  $z = 2E_h/\sqrt{s}$  bin limit (inclusive, constant bin width  $\Delta z = 0.01$ ), cross section value  $d\sigma_{K^\pm}/dz$  [fb], statistical uncertainty, positive systematic uncertainty, negative systematic uncertainty. The uncertainties do not include the uncertainty on the normalization constant (1.4%).

|      |              |           |             |             |
|------|--------------|-----------|-------------|-------------|
| 0.20 | 6.3738e + 06 | 4.0e + 03 | 1.431e + 05 | 1.432e + 05 |
| 0.21 | 5.9816e + 06 | 3.9e + 03 | 1.397e + 05 | 1.397e + 05 |
| 0.22 | 5.5913e + 06 | 3.7e + 03 | 1.281e + 05 | 1.281e + 05 |
| 0.23 | 5.2343e + 06 | 3.6e + 03 | 1.212e + 05 | 1.212e + 05 |
| 0.24 | 4.9066e + 06 | 3.5e + 03 | 1.186e + 05 | 1.186e + 05 |
| 0.25 | 4.5784e + 06 | 3.3e + 03 | 1.164e + 05 | 1.165e + 05 |
| 0.26 | 4.2568e + 06 | 3.2e + 03 | 1.073e + 05 | 1.074e + 05 |
| 0.27 | 3.9475e + 06 | 3.1e + 03 | 1.013e + 05 | 1.013e + 05 |
| 0.28 | 3.6589e + 06 | 3.0e + 03 | 9.12e + 04  | 9.11e + 04  |
| 0.29 | 3.3960e + 06 | 2.9e + 03 | 9.07e + 04  | 9.06e + 04  |

|      |                |             |              |              |
|------|----------------|-------------|--------------|--------------|
| 0.30 | $3.1583e + 06$ | $2.7e + 03$ | $8.59e + 04$ | $8.58e + 04$ |
| 0.31 | $2.9480e + 06$ | $2.6e + 03$ | $8.58e + 04$ | $8.58e + 04$ |
| 0.32 | $2.7522e + 06$ | $2.6e + 03$ | $7.85e + 04$ | $7.85e + 04$ |
| 0.33 | $2.5661e + 06$ | $2.5e + 03$ | $7.58e + 04$ | $7.57e + 04$ |
| 0.34 | $2.3960e + 06$ | $2.4e + 03$ | $7.19e + 04$ | $7.18e + 04$ |
| 0.35 | $2.2389e + 06$ | $2.3e + 03$ | $6.88e + 04$ | $6.88e + 04$ |
| 0.36 | $2.0917e + 06$ | $2.2e + 03$ | $6.43e + 04$ | $6.42e + 04$ |
| 0.37 | $1.9487e + 06$ | $2.1e + 03$ | $6.29e + 04$ | $6.29e + 04$ |
| 0.38 | $1.8147e + 06$ | $2.1e + 03$ | $6.03e + 04$ | $6.03e + 04$ |
| 0.39 | $1.6906e + 06$ | $2.0e + 03$ | $5.64e + 04$ | $5.64e + 04$ |
| 0.40 | $1.5804e + 06$ | $1.9e + 03$ | $5.30e + 04$ | $5.29e + 04$ |
| 0.41 | $1.4802e + 06$ | $1.9e + 03$ | $5.31e + 04$ | $5.30e + 04$ |
| 0.42 | $1.3890e + 06$ | $1.8e + 03$ | $5.10e + 04$ | $5.10e + 04$ |
| 0.43 | $1.3000e + 06$ | $1.7e + 03$ | $4.85e + 04$ | $4.85e + 04$ |
| 0.44 | $1.2145e + 06$ | $1.7e + 03$ | $4.65e + 04$ | $4.65e + 04$ |
| 0.45 | $1.1338e + 06$ | $1.6e + 03$ | $4.42e + 04$ | $4.42e + 04$ |
| 0.46 | $1.0588e + 06$ | $1.6e + 03$ | $4.06e + 04$ | $4.06e + 04$ |
| 0.47 | $9.860e + 05$  | $1.5e + 03$ | $4.00e + 04$ | $4.01e + 04$ |
| 0.48 | $9.193e + 05$  | $1.5e + 03$ | $3.71e + 04$ | $3.72e + 04$ |
| 0.49 | $8.574e + 05$  | $1.4e + 03$ | $3.61e + 04$ | $3.62e + 04$ |
| 0.50 | $7.999e + 05$  | $1.4e + 03$ | $3.19e + 04$ | $3.19e + 04$ |
| 0.51 | $7.486e + 05$  | $1.3e + 03$ | $3.09e + 04$ | $3.10e + 04$ |
| 0.52 | $7.005e + 05$  | $1.3e + 03$ | $2.99e + 04$ | $3.00e + 04$ |
| 0.53 | $6.561e + 05$  | $1.2e + 03$ | $2.72e + 04$ | $2.73e + 04$ |
| 0.54 | $6.135e + 05$  | $1.2e + 03$ | $2.56e + 04$ | $2.57e + 04$ |
| 0.55 | $5.738e + 05$  | $1.2e + 03$ | $2.36e + 04$ | $2.37e + 04$ |
| 0.56 | $5.350e + 05$  | $1.1e + 03$ | $2.29e + 04$ | $2.30e + 04$ |
| 0.57 | $4.979e + 05$  | $1.1e + 03$ | $2.04e + 04$ | $2.05e + 04$ |
| 0.58 | $4.628e + 05$  | $1.0e + 03$ | $1.93e + 04$ | $1.94e + 04$ |
| 0.59 | $4.306e + 05$  | $1.0e + 03$ | $2.07e + 04$ | $2.07e + 04$ |

|      |              |           |             |             |
|------|--------------|-----------|-------------|-------------|
| 0.60 | 4.0115e + 05 | 9.7e + 02 | 1.637e + 04 | 1.643e + 04 |
| 0.61 | 3.7227e + 05 | 9.4e + 02 | 1.554e + 04 | 1.559e + 04 |
| 0.62 | 3.4598e + 05 | 9.1e + 02 | 1.355e + 04 | 1.360e + 04 |
| 0.63 | 3.2109e + 05 | 8.8e + 02 | 1.420e + 04 | 1.426e + 04 |
| 0.64 | 2.9735e + 05 | 8.5e + 02 | 1.294e + 04 | 1.305e + 04 |
| 0.65 | 2.7474e + 05 | 8.1e + 02 | 1.327e + 04 | 1.341e + 04 |
| 0.66 | 2.5378e + 05 | 7.8e + 02 | 1.366e + 04 | 1.385e + 04 |
| 0.67 | 2.3466e + 05 | 7.6e + 02 | 1.192e + 04 | 1.219e + 04 |
| 0.68 | 2.1668e + 05 | 7.3e + 02 | 1.262e + 04 | 1.292e + 04 |
| 0.69 | 1.9908e + 05 | 7.0e + 02 | 1.145e + 04 | 1.182e + 04 |
| 0.70 | 1.8419e + 05 | 6.8e + 02 | 1.233e + 04 | 1.271e + 04 |
| 0.71 | 1.6900e + 05 | 6.5e + 02 | 1.239e + 04 | 1.278e + 04 |
| 0.72 | 1.5588e + 05 | 6.3e + 02 | 1.137e + 04 | 1.180e + 04 |
| 0.73 | 1.4314e + 05 | 6.1e + 02 | 1.122e + 04 | 1.167e + 04 |
| 0.74 | 1.3119e + 05 | 5.8e + 02 | 1.155e + 04 | 1.197e + 04 |
| 0.75 | 1.1989e + 05 | 5.6e + 02 | 1.094e + 04 | 1.136e + 04 |
| 0.76 | 1.1004e + 05 | 5.4e + 02 | 1.075e + 04 | 1.116e + 04 |
| 0.77 | 9.973e + 04  | 5.1e + 02 | 9.89e + 03  | 1.031e + 04 |
| 0.78 | 9.104e + 04  | 5.0e + 02 | 8.95e + 03  | 9.38e + 03  |
| 0.79 | 8.287e + 04  | 4.8e + 02 | 9.14e + 03  | 9.53e + 03  |
| 0.80 | 7.481e + 04  | 4.6e + 02 | 8.87e + 03  | 9.24e + 03  |
| 0.81 | 6.754e + 04  | 4.4e + 02 | 8.17e + 03  | 8.54e + 03  |
| 0.82 | 6.080e + 04  | 4.2e + 02 | 7.90e + 03  | 8.24e + 03  |
| 0.83 | 5.431e + 04  | 4.0e + 02 | 7.16e + 03  | 7.51e + 03  |
| 0.84 | 4.739e + 04  | 3.7e + 02 | 6.87e + 03  | 7.18e + 03  |
| 0.85 | 4.218e + 04  | 3.6e + 02 | 6.69e + 03  | 6.98e + 03  |
| 0.86 | 3.698e + 04  | 3.4e + 02 | 6.21e + 03  | 6.49e + 03  |
| 0.87 | 3.238e + 04  | 3.2e + 02 | 5.70e + 03  | 5.97e + 03  |
| 0.88 | 2.787e + 04  | 3.1e + 02 | 5.12e + 03  | 5.39e + 03  |
| 0.89 | 2.340e + 04  | 2.8e + 02 | 5.09e + 03  | 5.32e + 03  |
| 0.90 | 2.003e + 04  | 2.7e + 02 | 4.59e + 03  | 4.81e + 03  |
| 0.91 | 1.700e + 04  | 2.6e + 02 | 4.62e + 03  | 4.83e + 03  |
| 0.92 | 1.424e + 04  | 2.4e + 02 | 4.01e + 03  | 4.22e + 03  |
| 0.93 | 1.175e + 04  | 2.4e + 02 | 3.81e + 03  | 4.01e + 03  |
| 0.94 | 8.81e + 03   | 2.2e + 02 | 3.56e + 03  | 3.75e + 03  |
| 0.95 | 6.37e + 03   | 2.1e + 02 | 3.40e + 03  | 3.59e + 03  |
| 0.96 | 4.67e + 03   | 2.2e + 02 | 3.50e + 03  | 3.69e + 03  |
| 0.97 | 5.92e + 03   | 4.4e + 02 | 7.34e + 03  | 7.72e + 03  |

#### FRACTIONS OF PIONS PRODUCED IN STRONG AND WEAK DECAYS

Low  $z = 2E_h/\sqrt{s}$  bin limit (inclusive, width  $\Delta z = 0.01$ ), fraction from strong decays, uncertainty of fraction from strong decays (stat.), fraction from weak decays, uncertainty of fraction from weak decays (stat.).

|      |         |         |         |         |
|------|---------|---------|---------|---------|
| 0.20 | 0.70372 | 0.00027 | 0.29628 | 0.00015 |
| 0.21 | 0.70370 | 0.00028 | 0.29630 | 0.00016 |
| 0.22 | 0.70441 | 0.00030 | 0.29559 | 0.00017 |
| 0.23 | 0.70457 | 0.00032 | 0.29543 | 0.00018 |
| 0.24 | 0.70528 | 0.00033 | 0.29472 | 0.00019 |
| 0.25 | 0.70600 | 0.00035 | 0.29400 | 0.00020 |
| 0.26 | 0.70690 | 0.00037 | 0.29310 | 0.00021 |
| 0.27 | 0.70820 | 0.00039 | 0.29180 | 0.00022 |
| 0.28 | 0.70898 | 0.00041 | 0.29102 | 0.00023 |
| 0.29 | 0.71022 | 0.00043 | 0.28978 | 0.00024 |
| 0.30 | 0.71210 | 0.00045 | 0.28790 | 0.00025 |
| 0.31 | 0.71324 | 0.00048 | 0.28676 | 0.00026 |
| 0.32 | 0.71445 | 0.00050 | 0.28555 | 0.00027 |
| 0.33 | 0.71617 | 0.00053 | 0.28383 | 0.00029 |
| 0.34 | 0.71783 | 0.00055 | 0.28217 | 0.00030 |
| 0.35 | 0.71995 | 0.00058 | 0.28005 | 0.00031 |
| 0.36 | 0.72156 | 0.00061 | 0.27844 | 0.00033 |
| 0.37 | 0.72394 | 0.00064 | 0.27606 | 0.00034 |
| 0.38 | 0.72594 | 0.00067 | 0.27406 | 0.00035 |
| 0.39 | 0.72880 | 0.00070 | 0.27120 | 0.00037 |
| 0.40 | 0.73133 | 0.00074 | 0.26867 | 0.00038 |
| 0.41 | 0.73413 | 0.00077 | 0.26587 | 0.00040 |
| 0.42 | 0.73724 | 0.00081 | 0.26276 | 0.00041 |
| 0.43 | 0.74037 | 0.00085 | 0.25963 | 0.00043 |
| 0.44 | 0.74316 | 0.00090 | 0.25684 | 0.00045 |
| 0.45 | 0.74764 | 0.00094 | 0.25236 | 0.00046 |
| 0.46 | 0.75143 | 0.00099 | 0.24857 | 0.00048 |
| 0.47 | 0.7550  | 0.0010  | 0.24499 | 0.00050 |
| 0.48 | 0.7593  | 0.0011  | 0.24072 | 0.00052 |
| 0.49 | 0.7640  | 0.0012  | 0.23598 | 0.00054 |
| 0.50 | 0.7686  | 0.0012  | 0.23138 | 0.00056 |
| 0.51 | 0.7738  | 0.0013  | 0.22623 | 0.00058 |
| 0.52 | 0.7789  | 0.0014  | 0.22105 | 0.00060 |
| 0.53 | 0.7857  | 0.0014  | 0.21430 | 0.00061 |
| 0.54 | 0.7915  | 0.0015  | 0.20853 | 0.00063 |
| 0.55 | 0.7990  | 0.0016  | 0.20096 | 0.00065 |
| 0.56 | 0.8056  | 0.0017  | 0.19442 | 0.00067 |
| 0.57 | 0.8121  | 0.0018  | 0.18794 | 0.00069 |
| 0.58 | 0.8198  | 0.0019  | 0.18025 | 0.00071 |
| 0.59 | 0.8270  | 0.0020  | 0.17301 | 0.00072 |

|      |        |        |         |         |
|------|--------|--------|---------|---------|
| 0.60 | 0.8369 | 0.0021 | 0.16311 | 0.00073 |
| 0.61 | 0.8444 | 0.0022 | 0.15561 | 0.00075 |
| 0.62 | 0.8528 | 0.0023 | 0.14724 | 0.00076 |
| 0.63 | 0.8608 | 0.0025 | 0.13918 | 0.00078 |
| 0.64 | 0.8700 | 0.0026 | 0.12997 | 0.00079 |
| 0.65 | 0.8777 | 0.0028 | 0.12226 | 0.00080 |
| 0.66 | 0.8859 | 0.0029 | 0.11411 | 0.00081 |
| 0.67 | 0.8929 | 0.0031 | 0.10710 | 0.00083 |
| 0.68 | 0.9007 | 0.0033 | 0.09934 | 0.00084 |
| 0.69 | 0.9104 | 0.0035 | 0.08956 | 0.00083 |
| 0.70 | 0.9159 | 0.0037 | 0.08407 | 0.00085 |
| 0.71 | 0.9245 | 0.0040 | 0.07551 | 0.00085 |
| 0.72 | 0.9310 | 0.0042 | 0.06899 | 0.00085 |
| 0.73 | 0.9380 | 0.0045 | 0.06201 | 0.00085 |
| 0.74 | 0.9451 | 0.0047 | 0.05492 | 0.00084 |
| 0.75 | 0.9524 | 0.0051 | 0.04760 | 0.00083 |
| 0.76 | 0.9594 | 0.0054 | 0.04056 | 0.00081 |
| 0.77 | 0.9653 | 0.0057 | 0.03469 | 0.00079 |
| 0.78 | 0.9693 | 0.0061 | 0.03074 | 0.00079 |
| 0.79 | 0.9740 | 0.0065 | 0.02597 | 0.00077 |
| 0.80 | 0.9786 | 0.0070 | 0.02145 | 0.00074 |
| 0.81 | 0.9835 | 0.0075 | 0.01653 | 0.00069 |
| 0.82 | 0.9868 | 0.0080 | 0.01320 | 0.00066 |
| 0.83 | 0.9901 | 0.0086 | 0.00989 | 0.00061 |
| 0.84 | 0.9919 | 0.0093 | 0.00809 | 0.00060 |
| 0.85 | 0.993  | 0.010  | 0.00677 | 0.00058 |
| 0.86 | 0.995  | 0.011  | 0.00521 | 0.00056 |
| 0.87 | 0.996  | 0.012  | 0.00364 | 0.00051 |
| 0.88 | 0.998  | 0.013  | 0.00231 | 0.00044 |
| 0.89 | 0.999  | 0.014  | 0.00130 | 0.00036 |
| 0.90 | 0.999  | 0.015  | 0.00060 | 0.00027 |
| 0.91 | 1.000  | 0.017  | 0.00015 | 0.00015 |
| 0.92 | 1.000  | 0.019  | 0.00035 | 0.00025 |
| 0.93 | 1.000  | 0.021  | 0.00022 | 0.00022 |
| 0.94 | 1.000  | 0.024  | 0.0     | 0.0     |
| 0.95 | 1.000  | 0.028  | 0.0     | 0.0     |
| 0.96 | 1.000  | 0.033  | 0.0     | 0.0     |
| 0.97 | 1.000  | 0.030  | 0.0     | 0.0     |

# FRACTIONS OF KAONS PRODUCED IN STRONG AND WEAK DECAYS

Low  $z = 2E_h/\sqrt{s}$  bin limit (inclusive, width  $\Delta z = 0.01$ ), fraction from strong decays, uncertainty of fraction from strong decays (stat.), fraction from weak decays, uncertainty of fraction from weak decays (stat.).

|      |         |         |         |         |
|------|---------|---------|---------|---------|
| 0.20 | 0.57237 | 0.00040 | 0.42763 | 0.00033 |
| 0.21 | 0.56212 | 0.00041 | 0.43788 | 0.00035 |
| 0.22 | 0.55324 | 0.00043 | 0.44676 | 0.00037 |
| 0.23 | 0.54636 | 0.00044 | 0.45364 | 0.00039 |
| 0.24 | 0.54088 | 0.00046 | 0.45912 | 0.00041 |
| 0.25 | 0.53576 | 0.00047 | 0.46424 | 0.00043 |
| 0.26 | 0.53209 | 0.00049 | 0.46791 | 0.00045 |
| 0.27 | 0.52874 | 0.00050 | 0.47126 | 0.00047 |
| 0.28 | 0.52551 | 0.00052 | 0.47449 | 0.00049 |
| 0.29 | 0.52380 | 0.00054 | 0.47620 | 0.00051 |
| 0.30 | 0.52146 | 0.00056 | 0.47854 | 0.00053 |
| 0.31 | 0.52045 | 0.00058 | 0.47955 | 0.00055 |
| 0.32 | 0.51946 | 0.00060 | 0.48054 | 0.00057 |
| 0.33 | 0.51865 | 0.00063 | 0.48135 | 0.00060 |
| 0.34 | 0.51752 | 0.00065 | 0.48248 | 0.00062 |
| 0.35 | 0.51751 | 0.00068 | 0.48249 | 0.00065 |
| 0.36 | 0.51857 | 0.00070 | 0.48143 | 0.00067 |
| 0.37 | 0.51760 | 0.00073 | 0.48240 | 0.00070 |
| 0.38 | 0.51807 | 0.00076 | 0.48193 | 0.00072 |
| 0.39 | 0.51960 | 0.00079 | 0.48040 | 0.00075 |
| 0.40 | 0.52046 | 0.00082 | 0.47954 | 0.00078 |
| 0.41 | 0.52136 | 0.00086 | 0.47864 | 0.00081 |
| 0.42 | 0.52224 | 0.00089 | 0.47776 | 0.00084 |
| 0.43 | 0.52316 | 0.00093 | 0.47684 | 0.00087 |
| 0.44 | 0.52664 | 0.00097 | 0.47336 | 0.00091 |
| 0.45 | 0.5284  | 0.0010  | 0.47161 | 0.00094 |
| 0.46 | 0.5303  | 0.0011  | 0.46975 | 0.00098 |
| 0.47 | 0.5343  | 0.0011  | 0.4657  | 0.0010  |
| 0.48 | 0.5351  | 0.0012  | 0.4649  | 0.0011  |
| 0.49 | 0.5389  | 0.0012  | 0.4611  | 0.0011  |
| 0.50 | 0.5432  | 0.0013  | 0.4568  | 0.0011  |
| 0.51 | 0.5459  | 0.0013  | 0.4541  | 0.0012  |
| 0.52 | 0.5500  | 0.0014  | 0.4500  | 0.0012  |
| 0.53 | 0.5572  | 0.0015  | 0.4428  | 0.0013  |
| 0.54 | 0.5637  | 0.0016  | 0.4363  | 0.0013  |
| 0.55 | 0.5703  | 0.0016  | 0.4297  | 0.0014  |
| 0.56 | 0.5786  | 0.0017  | 0.4214  | 0.0014  |
| 0.57 | 0.5855  | 0.0018  | 0.4145  | 0.0015  |
| 0.58 | 0.5938  | 0.0019  | 0.4062  | 0.0015  |
| 0.59 | 0.6042  | 0.0021  | 0.3958  | 0.0016  |

|      |        |        |         |         |
|------|--------|--------|---------|---------|
| 0.60 | 0.6130 | 0.0022 | 0.3870  | 0.0016  |
| 0.61 | 0.6235 | 0.0023 | 0.3765  | 0.0017  |
| 0.62 | 0.6347 | 0.0025 | 0.3653  | 0.0017  |
| 0.63 | 0.6473 | 0.0026 | 0.3527  | 0.0018  |
| 0.64 | 0.6599 | 0.0028 | 0.3401  | 0.0018  |
| 0.65 | 0.6717 | 0.0030 | 0.3283  | 0.0019  |
| 0.66 | 0.6876 | 0.0032 | 0.3124  | 0.0019  |
| 0.67 | 0.6949 | 0.0034 | 0.3051  | 0.0020  |
| 0.68 | 0.7101 | 0.0036 | 0.2899  | 0.0020  |
| 0.69 | 0.7262 | 0.0039 | 0.2738  | 0.0021  |
| 0.70 | 0.7419 | 0.0042 | 0.2581  | 0.0021  |
| 0.71 | 0.7562 | 0.0045 | 0.2438  | 0.0021  |
| 0.72 | 0.7670 | 0.0048 | 0.2330  | 0.0022  |
| 0.73 | 0.7867 | 0.0052 | 0.2133  | 0.0022  |
| 0.74 | 0.8011 | 0.0056 | 0.1989  | 0.0023  |
| 0.75 | 0.8161 | 0.0060 | 0.1839  | 0.0023  |
| 0.76 | 0.8340 | 0.0064 | 0.1660  | 0.0023  |
| 0.77 | 0.8445 | 0.0070 | 0.1555  | 0.0024  |
| 0.78 | 0.8611 | 0.0075 | 0.1389  | 0.0024  |
| 0.79 | 0.8806 | 0.0082 | 0.1194  | 0.0023  |
| 0.80 | 0.8921 | 0.0089 | 0.1079  | 0.0024  |
| 0.81 | 0.9087 | 0.0095 | 0.0913  | 0.0023  |
| 0.82 | 0.926  | 0.010  | 0.0742  | 0.0022  |
| 0.83 | 0.936  | 0.011  | 0.0637  | 0.0022  |
| 0.84 | 0.948  | 0.012  | 0.0524  | 0.0021  |
| 0.85 | 0.957  | 0.013  | 0.0426  | 0.0020  |
| 0.86 | 0.970  | 0.015  | 0.0303  | 0.0019  |
| 0.87 | 0.980  | 0.016  | 0.0205  | 0.0016  |
| 0.88 | 0.980  | 0.017  | 0.0202  | 0.0018  |
| 0.89 | 0.985  | 0.019  | 0.0152  | 0.0017  |
| 0.90 | 0.991  | 0.021  | 0.0094  | 0.0015  |
| 0.91 | 0.9949 | 0.022  | 0.0051  | 0.0011  |
| 0.92 | 0.9959 | 0.025  | 0.0041  | 0.0012  |
| 0.93 | 0.9968 | 0.028  | 0.0032  | 0.0011  |
| 0.94 | 0.9979 | 0.032  | 0.0021  | 0.0010  |
| 0.95 | 0.9993 | 0.037  | 0.00070 | 0.00070 |
| 0.96 | 1.000  | 0.044  | 0.0     | 0.0     |

### CONTRIBUTIONS TO SYSTEMATIC UNCERTAINTIES

Figures 1 a) and b) show different contributions to the systematic uncertainties for the final charge-integrated pion (a) and kaon (b) cross sections in a stacked plot. The uncertainty on the normalization constant (1.4%) is not shown.



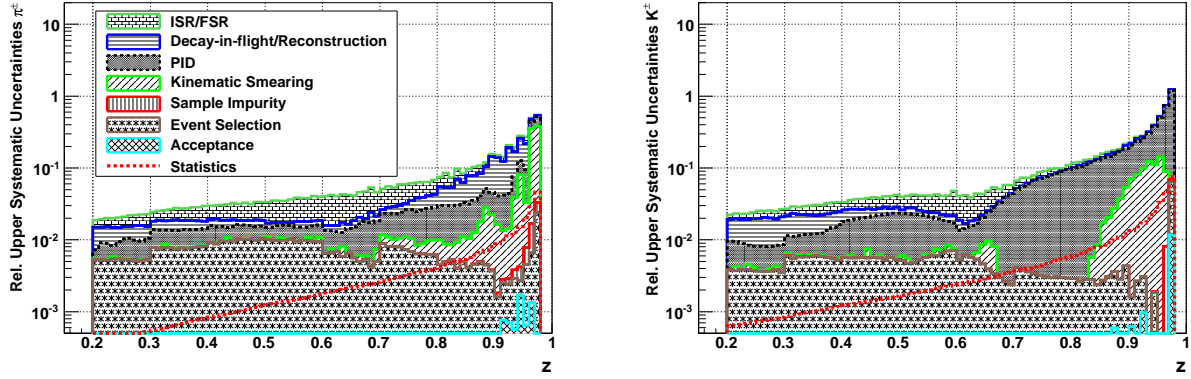

FIG. 1: Stacked plot of the increase of relative systematic uncertainties due to each correction step, for pions (a) and kaons (b). The individual contributions are particle identification (solid gray), sample impurity (vertical lines), momentum smearing (oblique lines), decay-in-flight and reconstruction (horizontal lines), event/track selection (star hatch), acceptance (cross hatch) and initial/final state photon radiation (brick hatch). The relative statistical uncertainty is shown in red dashes. The uncertainty on the normalization constant (1.4%) is not shown.

### COMPARISON OF MEASUREMENT RESULTS WITH MONTE CARLO GENERATED CROSS SECTIONS

The final charge-integrated pion and kaon cross sections,  $d\sigma_{h^\pm}/dz$  with  $z = 2E_h/\sqrt{s}$  and  $h^\pm = \{\pi^\pm, K^\pm\}$ , are compared with cross sections from the Belle MC and other MC samples generated with the PYTHIA 6.205 generator for  $e^+e^- \rightarrow q\bar{q}$  events, where  $q = \{u, d, s, c\}$ , at Belle center-of-mass energy. PYTHIA parameter sets as used by high-energy experiments like CDF, ATLAS and ALEPH are studied. Figure 2 shows ratios of MC over experimental data cross sections for pions (left) and kaons (right) with statistical and systematic uncertainties combined and propagated.

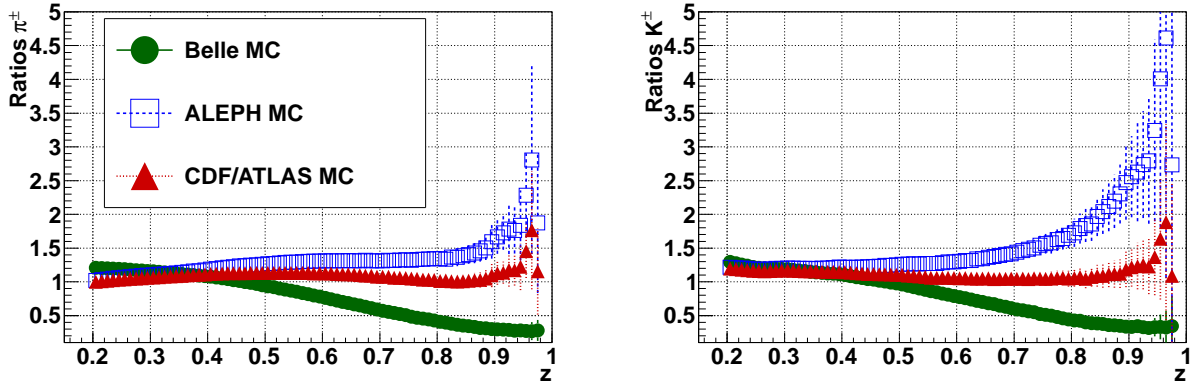

FIG. 2: Ratios between PYTHIA Monte Carlo and experimental data cross sections for pions (left) and kaons (right), for the Belle MC (circles), ALEPH (boxes) and CDF/ATLAS parameter sets (triangles).

### COMPARISON OF KAON CROSS SECTIONS WITH WORLD NORMALIZED CROSS SECTION DATA

The final charge-integrated kaon cross sections  $d\sigma_{K^\pm}/dz$  with  $z = 2E_h/\sqrt{s}$  are compared with normalized kaon cross sections  $1/\sigma_{\text{tot.had.}} \times d\sigma_{K^\pm}/dz$  from LEP and SLC experiments as well as from other, lower energy  $e^+e^-$  experiments from Refs. [1–7] in Fig. 3.

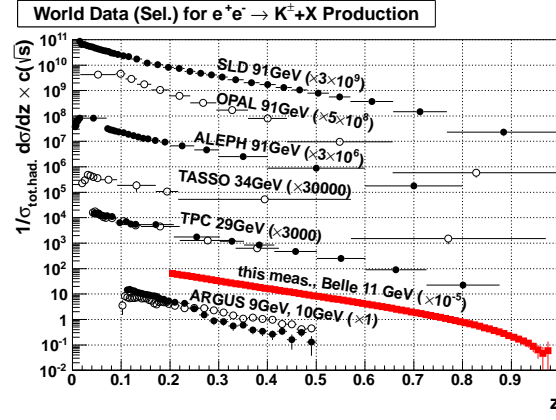

FIG. 3: Charge-integrated normalized kaon production cross sections from selected measurements and the Belle results. For better visibility all data sets are scaled by arbitrary numbers (indicated between parentheses). Statistical and systematic uncertainties are added in quadrature.

- 
- [1] R. Barate *et al.* (ALEPH Collaboration), Phys. Rep. **294**, 1 (1998).
  - [2] R. Akers *et al.* (OPAL Collaboration), Z. Phys. C **63**, 181 (1994).
  - [3] K. Abe *et al.* (SLD Collaboration), Phys. Rev. D **69**, 072003 (2004).
  - [4] H. Albrecht *et al.* (ARGUS Collaboration), Z. Phys. C **44**, 547 (1989).
  - [5] W. Braunschweig *et al.* (TASSO Collaboration), Z. Phys. C **42**, 189 (1989).
  - [6] H. Aihara *et al.* (TPC/Two Gamma Collaboration), Phys. Rev. Lett. **52**, 577 (1984).
  - [7] H. Aihara *et al.* (TPC/Two Gamma Collaboration), Phys. Rev. Lett. **61**, 1263 (1988).
